# Supplementary material for: Evaluating Metrics for Bias in Word Embeddings
Source: arXiv:2111.07864 source file (2024-09-12)
Supplement: Supplementary file 1 [file appendix.tex]

\setcounter{section}{0}

\section{dummy}
